# Supplementary material for: Language model compression with weighted low-rank factorization
Source: arXiv:2207.00112 source file (2022-06-30)
Supplement: Supplementary file 1 [file add.tex]

\begin{align}
{g_i} = ({\sigma _{im - m + 1,...,}}{\sigma _{im}}) 
\label{equ:gi}\\
{{\bar \Sigma }_i} = [{g_1},...,{g_i} = \vec 0,...,{g_{r/m}}] \label{equ:sigmai}
\end{align}

The factorization of a rank-$r$ matrix $W$ retain only the $r$ columns of $U$ and $V$, associated with non-zero singular values: ${\sigma _1} \ge {\sigma _2} \ge  \cdots {\sigma _r} > 0$. 
The low-rank approximation with target rank $l$ is achieved by setting zeros to the  last $r-l$ singular values.
The reconstruction of matrix $A$ can also be viewed rank revealing decomposition:
\begin{equation}
    %A=\sum_{k=1}^r \sigma_k u_k v_k^T,
    ||W||_F=\sum_{k=1}^r \sigma_k^2
    \label{equ:rank_decomposition}
\end{equation}
where $u_k$ and $v_k$ is the $k$th column of $V$.\yh{I do not quite understand the notations here}
For $i<j$, column $i$ will be more important in the matrix reconstruction process than column $j$, since ${\sigma_i > {\sigma_j}}$. 
Ideally, setting $\sigma_i$ to zero is supposed to cause larger reconstruction error and result in worse final performance than setting $\sigma_j$ to zero. 
Therefore,
